# Supplementary material for: A stochastic and dynamical view of pluripotency in mouse embryonic stem cells
Source: arXiv:1710.08542 source file (2017-10-23)
Supplement: Supplementary file 1 [file SI.pdf]

# Supplementary Information

Yen Ting Lin,[1, 2] Peter G. Hufton,[2] Esther J. Lee,[3] and Davit A. Potoyan[4]

[1] *T-6 and Center for Nonlinear Studies, Los Alamos National Laboratory, Los Alamos, NM 87545, USA*
[2] *School of Physics and Astronomy, The University of Manchester, Manchester, M13 9PL, UK*
[3] *Department of Bioengineering, Rice University, Houston, TX 77005, USA*
[4] *Department of Chemistry, Iowa State University, Ames, IA 50011, USA*

(Dated: April 11, 2017)

## I. METHODS

**Individual-based model.** We begin by constructing a individual-based model describing stochastic transitions between discrete molecular populations and discrete genetic states. In this model, reactant species are well-mixed and no spatial information is considered. Genes *produce* transcription factors (TFs) in a single-step reaction with a given production rate $\tilde{\alpha}$ [1]. We use letters decorated by a tilde symbol to denote the reaction rates in the individual-based setting (parameters will be renormalized; see next section). TFs *degrade* at a uniform constant rate $\tilde{\gamma}$. TFs regulate the production rate of other genes by *binding to* the promoter sites of regulated genes. The regulatory network is chosen to be a twelve-node network inferred from experiments by Dunn *et al.* [2], summarized in Fig. 1 of main text. To sum up, there are four reactions for each pair of gene and TF: (1) production of the TF, (2) degradation of TF, and (3) binding and (4) unbinding events of the TF.

To model cooperative binding, we assume each gene has $n$ promoter sites which can be bound by its regulating TFs. We set binding rates, $\tilde{k}_{on}$ (respectively, unbinding rates, $\tilde{k}_{\text{off}}$) per individual TF molecule to be uniform among all genes in the network. This assumption can be relaxed further to closer approximate the constraints. Depending on whether the promoter sites are occupied by activators or repressors, each gene can be in one of three states: activated, repressed or free. Detailed descriptions of the regulation are described below and summarized in Fig. 1 of main text. When a gene is only regulated by activators: The production rate of a free or partially bound gene is set to 0, and the transcription rate of a gene fully bound by $n$ (identical or different types of) activators is set to $\tilde{\alpha}_{\max}$. When a gene is only regulated by repressors: The production rate of a free or partially bound gene is set to $\tilde{\alpha}_{\max}$, and the production rate of a gene fully bound by $n$ (identical or different types of) repressors is set to 0. When a gene can be both regulated by activators and repressors: If the gene is fully bound by $n$ (identical or different types of) activators, the production rate is $\tilde{\alpha}_{\max}$. If the gene is fully bound by $n$ (identical or different types of) repressors, the production rate is 0. If the gene is neither bound to $n$ activators or repressors, the production rate is set to $\tilde{\alpha}_m \in [0, \tilde{\alpha}_{\max}]$, which is another model parameter.

**Non-dimensionalization of the model parameters.** Given a fixed genetic configuration, the production and degradation for a specific TF comprises a random birth and death process [3]. Without the binding and unbinding events, the population of each of the TFs would converge to a vicinity of a population $\approx \tilde{\alpha}/\tilde{\gamma}$ [3, 4], where $\tilde{\alpha} \in \{0, \tilde{\alpha}_m, \tilde{\alpha}_{\max}\}$ is the rate with which the TF is produced. Consequently, each TF has a largest population scale $\Omega$ defined as $\tilde{\alpha}_{\max}/\tilde{\delta}$.

The population scale $\Omega \gg 1$ in the biologically relevant parameter regime. It is useful to renormalize the integer-valued TF population by the population scale and quantify the TF population by the resulting *population density* $x_i$. In addition, we choose to non-dimensionalize the time by the timescale of degradation, $\tilde{\gamma}^{-1}$. After the renormalization and non-dimensionalization, the renormalized model parameters are

$$\begin{aligned}
\alpha_{\max} &\equiv 1, && \text{(high production rate)},\\
\alpha_m &= \tilde{\alpha}_m \Omega^{-1} \tilde{\gamma}^{-1}, && \text{(low production rate)},\\
\gamma &\equiv 1, && \text{(degradation rate)},\\
k_{\text{on}} &= \tilde{k}_{\text{on}} \Omega \tilde{\gamma}^{-1}, && \text{(binding rate of TF)},\\
k_{\text{off}} &= \tilde{k}_{\text{off}} \tilde{\gamma}^{-1}, && \text{(unbinding rate of TF)}.
\end{aligned}$$

**Constructing the piecewise-deterministic Markov process (PDMP).** The individual-based model, a Markov jump process, is complex and no general technique exists to our knowledge to analytically investigate this type of systems. As the dimensionality of the system is high, numerically solving the chemical master equation governing the random process [3] becomes very inefficient. Efficient sampling the probability distribution numerically is needed. Because the biologically relevant population scale of each of the TFs is large (we set it to be $\Omega = 10^4$), it is not feasible to use standard continuous-time Monte Carlo [5, 6] sampling to infer the parameter regimes reproducing experimental results.

Recent studies on gene expression dynamics [7–12], have seen the emergence of a new framework using a piecewise-deterministic Markov process (PDMP) to approximate the individual-based model with a switching property. In this section, we briefly recapitulate the construction of the PDMP, as more thorough analysis can be found in the aforementioned references.

A PDMP is a process such that, in between discrete random switching events, the evolution of the process is deterministic. To construct the deterministic evolution of the TF populations, starting from the chemical master equations, we performed Kramers–Moyal expansion [3, 13] and only keep the first order of the expansion. The result is a standard Liouville's equation governing the *deterministic flow* of the distribution. The joint probability distribution of our model converges to the deterministic flow in a given genetic state and in the limit $\Omega \to \infty$ [13]. With the PDMP approach, the demographic noise originated from random birth-death events are neglected, so that the population density $x_i(t)$ of each TF evolves according to

$$\frac{\mathrm{d}}{\mathrm{d}t} x_i\left(t\right) = \alpha_i - x_i\left(t\right), \tag{2}$$

where $\alpha_i \in \{0, \alpha_m, 1\}$ is the production rate of the $i$th TF dependent on the $i$th gene's configuration of promoter sites. While the evolution of the TF population density is deterministic, the binding and unbinding events of the regulating TFs to their target genes are stochastic. For each of the gene, the reactions can be summarized as

$$G \underset{k_{\mathrm{off}}}{\overset{n\times k_{\mathrm{on}} x_i(t)}{\rightleftharpoons}} GP_i, \tag{3a}$$

$$GP_i \xrightarrow{(n-1)\times k_{\mathrm{on}} x_j(t)} GP_iP_j, \tag{3b}$$

$$GP_iP_j, \xrightarrow{k_{\mathrm{off}}} GP_i, \tag{3c}$$

$$GP_iP_j, \xrightarrow{k_{\mathrm{off}}} GP_j, \tag{3d}$$

$$\vdots$$

where $i, j$ runs over the set of regulating TFs of the genes. Note the mechanism is formulated as *parallel* binding to and unbinding from $n$ different promoter sites, rather than modeling sequential or site-specific binding.

We finally emphasize that the PDMP only retains the contribution of *switching noise* and ignores *demographic stochasticity* resulting from the discrete birth-death process. The PDMP is the limiting process when the population scale $\Omega \to \infty$ [10], and the error bound of the description can be rigorously derived to be $\mathcal{O}(\Omega^{-1})$ [14].

**Generating exact sample paths of the PDMP.** To simulate the stochastic gene switching, accurate waiting times must be generated. An established way to do so involves numerical integration of survival functions describing each potential transition [11]. In our case, the simple form of Eq. (2) allows us to efficiently generate waiting times without numerical integration. The TF density of a given type, with an initial condition $x_0$, is described by

$$x(t) = \alpha + (x_0 - \alpha)\exp\left(-t\right). \tag{4}$$

It follows that the survival function—the probability that the switching time is greater than time $t$—describing a genetic binding event is given by

$$\begin{aligned} S(t) &= \exp\left[-k_{\mathrm{on}} \int_0^t x(t')\,\mathrm{d}t'\right] \\ &= \exp\left\{-k_{\mathrm{on}}\left[\alpha t - \left(x_0 - \alpha\right)e^{-t} + x_0 - \alpha\right]\right\}. \end{aligned} \tag{5}$$

To use the inverse method, one generates a random number $u \sim \mathrm{Unif}\left(0,1\right)$ and equates it to Eq. (5). Solving this equation for $t$ gives the switching time. Although not solvable analytically, this equation can be solved numerically and with efficiency using the Newton–Raphson scheme.

For the case when the density is monotonically decreasing ($x_0 > \alpha$), a similar scheme [15] allows one to rigorously generate *exact* switching times. This involves generating two random numbers $u_1$, $u_2 \sim \mathrm{Unif}\left(0,1\right)$ such that the random time of a binding event $t$ is given by $t = \min(t_1, t_2)$ where

$$t_1 = \begin{cases} -\frac{1}{k_{\mathrm{on}}\alpha}\log u_1, & \text{if } \alpha \neq 0, \\ \infty, & \text{otherwise}, \end{cases} \tag{6a}$$

$$t_2 = \begin{cases} -\log\left[\frac{1}{k_{\mathrm{on}}}\left(x_0 - \alpha\right)^{-1}\log u_2 + 1\right], & \\ \qquad \text{if } u_2 > \exp\left[-k_{\mathrm{on}}\left(x_0 - \alpha\right)\right], & \\ \infty, \qquad \text{otherwise}. & \end{cases} \tag{6b}$$

Used together, we found these time-generating schemes provided a significant speed and accuracy advantage over the method involving numerical integration.

**Using the checkerboard diagram to infer the parameter regime.** After non-dimensionalizing the model there are four free parameters: $\rho_m$ as the intermediate production rate of those genes which are regulated by both activators and repressors, $k_{\text{on}}$, $k_{\text{off}}$ as the binding and unbinding rate of the TF to the promoter sites, and $n$ as the number of promoter sites per gene. To narrow down the parameter regime, we match our model predictions to the experimental findings of Dunn *et al.* [2] in which the authors measured the TF expression under various combination of external signals, i.e., LIF, CH, and PD. From simulation, we extract the binarized TF expression pattern under five distinct external signals, including LIF+2i, LIF+CH, LIF+PD, 2i, and none external driver are applied to the system.

We aim to match the model prediction to a twelve-by-five "checkerboard diagram" which records the experimentally measured expression pattern presented in Fig. 2 of main text. To achieve this goal, we performed a sweep in a vast parameter space: $\alpha_m \in [0, 1]$, $k_{\text{on}}, k_{\text{off}} \in [0, 110]$, and $n = 1, 2 \dots 5$. For each parameter set, we simulated $10^3$ PDMP sample paths for a time to sufficiently reflect the stationary state, and the average TF expression levels were recorded. Because of the non-dimensionalization, the expression level (the population density) of each TF is a real number in between 0 and 1. This results in a twelve-by-five real-valued matrix, which is binarized by a threshold. To find the optimal threshold, we use the number of discrepancies between the model prediction and the target matrix—the Hamming distance—as a quantitative measure. For each parameter set, an optimal threshold which minimizes the Hamming distance was then solved computationally, and the minimal Hamming distance was recorded and plotted in Fig. 2 as a "landscape" of how good the model captures the experimental results.

We found that for $n = 1$ and $n \geq 2$, the global minimal Hamming distance is 5 and 3 respectively. We chose $n = 2$ to present our follow-up analysis, as it incorporates the capacity of modeling cooperative binding which is often modeled phenomenologically. We find the Hamming distance can be constantly as small as 3 in a vast region in the space of binding/unbindnig rates when $\rho_m$ is small ($\lesssim 0.02$). Therefore, in the manuscript we present the landscape of a fast switching regime $k_{\text{on}} \approx 100$, an intermediate regime $k_{\text{on}} \approx 15$ and a slow switching regime $k_{\text{on}} \approx 3$.

**Model prediction of the TF expression.** We select three parameter sets which, each of which maximizes the agreement with the experimental results of Dunn *et al.* for a given rate of binding. These are denoted by the red dots in Fig. 2. For each parameter set and each of the possible combination of the external driver (LIF,CH,PD), we perform $10^5$ sample paths for a sufficiently long time to measure the marginal stationary distribution of the TF densities. To summarize the large data set of the TF densities under various conditions generated by the computational model, we rescale the marginal distributions so that their largest value is renormalized to be 1, and then visualize the results as heat maps in Fig. 3. The corresponding checkerboard diagrams are also generated and presented in Fig. 2.

**Check using the individual-based model.** For the three selected parameter sets, $10^4$ sample paths of a fully individual-based model were generated by standard kinetic Monte Carlo simulations [5, 6]. The population scale $\Omega$ for each TF is set to be $10^4$. A parallel analysis is carried out and the results are consistent with the predictions from using the PDMP. We report the results of the intermediate switching regime in Fig.4 .

**Visualizing the fluctuation in a lower dimension using principle component analysis (PCA).** While the joint probability distributions are measured by kinetic Monte Carlo sampling, the dimensionality of the dynamical system is very large: each TF has a real-valued density, and the gene controlling the transcription of the TF has a discrete genetic state (see Fig.1) Although Fig. 4 summarizes the marginal distributions of the real-valued TF density and contains rich information, it is desirable to visualize the results in a lower dimensional space to draw qualitative conclusions. To achieve this goal, we perform the standard principle component analysis [16]. We chose a baseline external condition to be LIF+2i; the first two principle components were computed. For the rest of the external conditions, the joint probability distributions are projected onto the plane spanned by these principle components; the results are presented in Fig. 7.

**Dynamical transitions between different external signals.** To investigate dynamical transitions when the external driving conditions (whether LIF, CH, and PD are present) change, we prepare $10^5$ independent sample paths with an initial external condition until the joint probability distribution converges to the stationary distribution. Then, the external condition is switched instantaneously to the second condition. We further evolve the dynamical system until stationarity for the second conditions is reached. The results are summarized in Fig. 5. To estimate the transition times between the stationary distributions with different external conditions, we measure the Jensen–Shannon distance of the marginal distribution of each TF density, at any given time during the transition to the final marginal distribution. We measure and report the first time when all 12 distances are below a threshold value of 0.3, presented in Fig. 6.

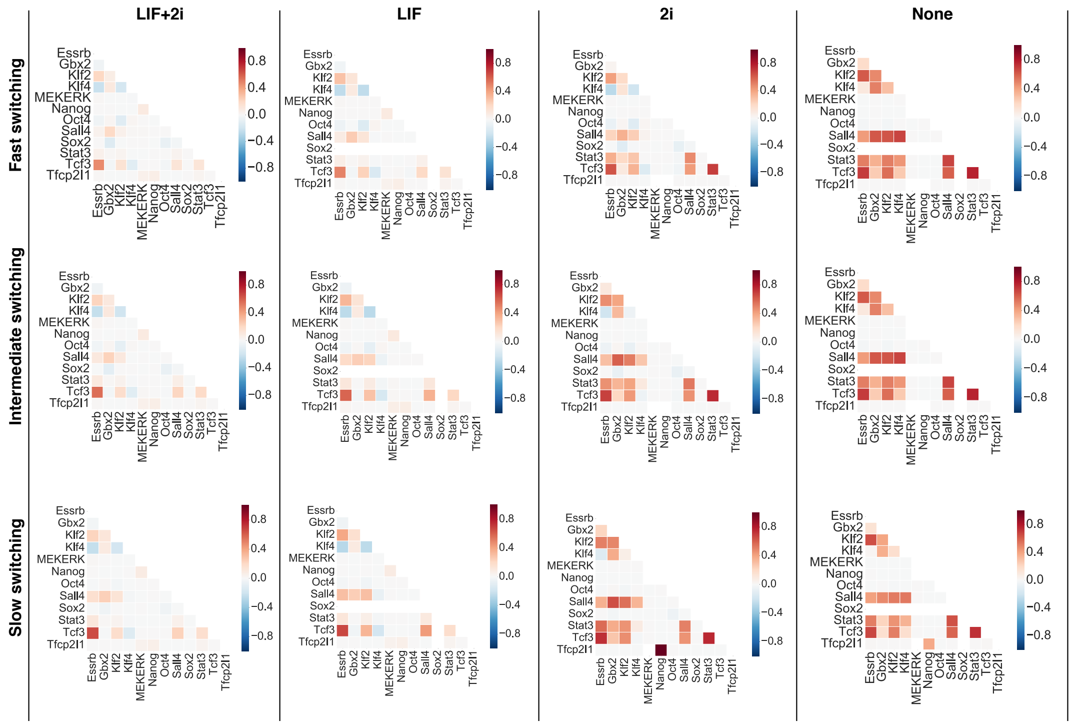


FIG. 1. Analyzing pairwise correlation patterns between different transcription factors under both different switching and signaling conditions.


[1] We remark that more detailed models involving intermediate transcription into and translation of mRNA [8, 9] can be included in this framework; We do not consider these more detailed reactions in this article.
[2] S.-J. Dunn, G. Martello, B. Yordanov, S. Emmott, and A. Smith, Science **344**, 1156 (2014).
[3] C. W. Gardiner *et al.*, *Handbook of stochastic methods*, Vol. 3 (Springer Berlin, 1985).
[4] T. G. Kurtz, Journal of Applied Probability **8**, 344 (1971).
[5] R. Schwartz, *Biological modeling and simulation: a survey of practical models, algorithms, and numerical methods* (MIT Press, 2008).
[6] D. T. Gillespie, The journal of physical chemistry **81**, 2340 (1977).
[7] D. A. Potoyan and P. G. Wolynes, The Journal of chemical physics **143**, 195101 (2015).
[8] Y. T. Lin and T. Galla, Journal of The Royal Society Interface **13**, 20150772 (2016).
[9] Y. T. Lin and C. R. Doering, Physical Review E **93**, 022409 (2016).
[10] P. G. Hufton, Y. T. Lin, T. Galla, and A. J. McKane, Physical Review E **93**, 052119 (2016).
[11] S. Zeiser, U. Franz, O. Wittich, and V. Liebscher, IET systems biology **2**, 113 (2008).
[12] S. Zeiser, U. Franz, and V. Liebscher, Journal of Mathematical Biology **60**, 207 (2010).
[13] T. G. Kurtz, Journal of applied Probability **7**, 49 (1970).
[14] T. Jahnke and M. Kreim, Multiscale Modeling & Simulation **10**, 1119 (2012).
[15] P. Bokes, J. R. King, A. T. Wood, and M. Loose, Bulletin of mathematical biology **75**, 351 (2013).
[16] I. Jolliffe, *Principal component analysis* (Wiley Online Library, 2002).
